# Supplementary material for: Guarantees for Comprehensive Simulation Assessment of Statistical Methods
Source: arXiv:2212.10042 source file (2024-09-09)
Supplement: Supplementary file 1 [file importance.tex]

\section{Importance Sampling}%
\label{sec:appendix-e}

For many-parameter problems, the methods described earlier in this document may require trillions of Monte Carlo simulations. In this section we will discuss a technique which can drastically reduce the number of simulations required.

Importance sampling is a famous technique, often used to efficiently sample low-probability events. This is moderately helpful in regions where Type I Error is small, but in fact the benefits from simulation \textit{re-use} across different values of $\theta$ are far greater. Because simulations can be re-weighted for re-use \textit{across different parameter values}, a massive parallel advantage can be gained.

We will use an approach inspired by defensive importance sampling \cite{owen2000safe}, with Veach's balance heuristic \cite{veach1995optimally}. The defensive element is that some (smaller number of) simulations will be drawn from the base Monte Carlo. This will bound the increments of our estimator, thus permitting a conformalized-tuning argument to prove Type I Error control for calibration.

The importance estimator will require the following quantities, which can be chosen using pilot simulations:

\begin{itemize}
    \item A collection of parameter targets $\theta_j$ for $j \in \{1,\ldots, J\}$ where we desire to establish control or upper bounds. We take $n_0$ Monte Carlo simulations under each $\theta_j$ (independently of the pilot simulations). These simulations may be correlated at different values of $j$'s, as long as each group with $j$ fixed is distributed i.i.d..
    \item A collection of additional parameter locations for taking importance samples: $\theta_k$ for $k \in {1, \ldots, K}$. %Assume that the first $J$ in this list are the target distribution parameters, so that Monte Carlo simulations may be considered a part of this simulation base.
    We will take $n_k$ simulations from each $\theta_k$. Unlike previously, ALL of these simulations should be independent of all other simulations.
    \item A collection of weights $w_{jk}$, for $j$ in $1, \ldots, J$ and $k$ in $0, 1, \ldots, K$. Importance sampling for $\theta_j$ will be performed with a deterministic mixture of the $\theta_k$ with weights $w_{jk}$ for $k \geq 1$, with weight
    $w_{k0}$ given to $\theta_j$'s own Monte Carlo simulations. Thus, we require $\sum \limits_{k=0}^J w_{jk} = 1$, and $0 \leq w_{jk} \leq 1$. %Observe that for $\theta_j$ with $j \leq J$, $w_{jj}$ is the proportion of the importance estimate which can be attributed to simple Monte Carlo samples from $\theta_j$.
\end{itemize}

The values $\theta_k$, $p_{jk}$ are assumed to be chosen beforehand on the basis of pilot simulations. Our goal is to reduce the number of total simulations necessary, by allowing $n_0$ to be small, and having the rest of the estimation done by a common set of simulations, yet keeping $w_{j0}$ large enough to recover strong guarantees.

Using Veach's balance heuristic \cite{veach1995optimally} and following Owen's recommendation to use a deterministic mixture \cite{owen2000safe} , the importance sampling estimator is defined as:

$$\widehat{f(\theta_j)}_{IS} := \sum \limits_{k=0}^K \frac{w_{jk}}{n_k} \sum \limits_{i=1}^{n_k}  \frac{P_j(X^k_i) F(X_{ik})}{\sum \limits_{m=0}^K w_{jm}P_m(X^k_i)}$$

where $X^k_i$ are the simulation data under $\theta_k$ for $k \geq 1$ and under $\theta_j$ for $k=0$, all of these simulations i.i.d.; $F(X^k_i)$ are the indicators for false rejection; and $P_j(X^k_i)$ are likelihoods of drawing dataset $(X^k_i)$ under $\theta_j$.

This estimator is unbiased, because it is an application of Veach's balance heuristic applied to the target integral $\int F(X_{i}) dP_j (X_{i})$.

We also show a proof here:

$$E\left[\sum \limits_{k=0}^K \frac{w_{jk}}{n_k} \sum \limits_{i=1}^{n_k}  \frac{P_j(X^k_i)F(X_{ik})}{\sum \limits_{m=0}^K w_{jm}P_m(X^k_i)}\right]$$

This expectation is an unbiased empirical evaluation of the expression below, if $k'$ were chosen at random from $1 \ldots K$ with probability $w_{jk}$:

$$= E\left[  \frac{P_j(X^{k'})F(X_{k'})}{\sum \limits_{m=0}^K w_{jm}P_m(X^{k'})}\right]$$

$$= \int \sum \limits_{k=0}^K w_{jk} P_{k(X^{k'})} \frac{P_j(X^{k'})F(X_{ik})}{\sum \limits_{m=0}^K w_{jm}P_m(X^{k'})}$$

$$= \int P_j(X^{k'})F(X_{ik}) = f(\theta_j)$$

\bigskip

We can also re-write this expression using likelihood ratios:

$$\widehat{f(\theta_j)}_{IS} := \sum \limits_{k=0}^K \frac{w_{jk}}{n_k} \sum \limits_{i=1}^{n_k}  \frac{P_j(X^k_i)F(X_{ik})}{\sum \limits_{m=0}^K w_{jm}P_m(X^k_i)} = \sum \limits_{k=0}^K \frac{w_{jk}}{n_k} \sum \limits_{i=1}^{n_k}  \frac{F(X_{ik})}{w_{j0} + \sum \limits_{m=1}^K w_{jm}\frac{P_m}{P_j}(X^k_i)}$$

Note that the increments of this expression are upper-bounded by $\frac{w_{jk}}{n_k w_{j0}}$. To achieve a calibration guarantee at target level $\alpha'$, it suffices to select $\hat{\lambda}$ such that

$\widehat{f(\theta_j)}_{IS} + \max_{j,k}\frac{w_{jk}}{n_k w_{j0}}< \alpha'$

Proof:

Our empirical process $\widehat{f_\lambda(\theta_j)}_{IS}$ can be re-indexed as a weighted average of  $I = \sum \limits_k n_{k}$  terms $F_{\lambda,y_i}$ which are nondecreasing functions of $\lambda$ (typically jumping from 0 to a fixed value), each having weight $w_{i} =\frac{w_{jk}}{n_k}$ such that $\sum \limits_{i=1}^I w_i = 1$. Next, generate a new independent element $Y$ by selecting $i'$ with probability $w_i$, and setting Y to an independent draw of $F_{\lambda,y_{i'}}$ .

Because Y is independent of the other simulations, by a calculation of the unbiasedness of the balance heuristic, notice that $E[f_{\hat{\lambda}}] =E[F_{\hat{\lambda},Y}]$ is equal to the average Type I Error of the calibration process.

However, conditionally on the index $i$ being assigned to $Y$, we may exchange $Y$ with $y_{i'}$ because they have the same distribution; thus

$$f_{\hat{\lambda}}(\theta_j)_{IS} = E[F_{\hat{\lambda},Y}] = E[F_{\hat{\lambda}:y_{i'} \rightarrow Y,y_{i'}}] = \sum \limits_i w_i E[ F_{\hat{\lambda}:y_{i} \rightarrow Y, y_i}]$$

Where $\hat{\lambda}:y_{i'} \rightarrow Y$ is the result from tuning with $Y$ replacing $y_i$.

However, by construction of the stopping rule, we have

$$\alpha' \geq \widehat{f_{\hat{\lambda}}(\theta_j)}_{IS} + \max_{j,k}\frac{w_{jk}}{n_k w_{j0}} = \sum \limits_{i} w_i F_{\hat{\lambda}, y_i} + \max_{j,k}\frac{w_{jk}}{n_k w_{j0}} \geq \sum \limits_{i} w_i F_{\hat{\lambda}:y_{i} \rightarrow Y, y_i}$$

Hence, adding an expectation on the right-hand-side, we recover 

$$f_{\hat{\lambda}}(\theta_j)_{IS} \leq \alpha'$$ and have the desired Type I Error control level. QED

This argument is similar to the control arguments provided in https://arxiv.org/abs/2208.02814, which also provides a similarly tight lower bound on the calibration. 
%We have lost a tiny bit of tightness, which we could probably recover by being a little more careful as we compare the worst-case effect of adding in Y. But I suppose this will do for now.

%\bigskip

%Note to add elsewhere to reference this section: Much can be done to improve simulation scaling. For example, Sklar (2021) discusses how using correlated random number generation can speed up computation. [None of our arguments require that simulations under $\theta_{j_1}$ and $\theta_{j_2}$, for $j_1 \neq j_2$, must be independent.] In Appendix E, we discuss an entirely different approach to use importance sampling for simultaneous simulation generation, with a generalized form of CSE.

%Note to add elsewhere re: calibration: it can generally be expected that this calibration setup will incentivize applicants to scale up their simulations appropriately, because the too-low simulation numbers cost the company by reducing power. Both bias and variability in the Type I Error of the selected $\lambda^*$ will harm power. But, both of these drawbacks can be mitigated and sent to 0 with additional simulations.
