# Supplementary material for: Guarantees for Comprehensive Simulation Assessment of Statistical Methods
Source: arXiv:2212.10042 source file (2024-09-09)
Supplement: Supplementary file 2 [file sequentialconditioning.tex]

\section{Sequential Conditioning}%
\label{sec:appendix-f}

In this section we extend CSE calibration for practical adaptive trials where difficulties in sample sizing and recruitment are expected, and where unplanned modifications may be necessary. 

Broadly, we separate the trial's adaptations into \textit{planned adaptations}, i.e. those which are described and committed-to in the trial protocol, and \textit{unplanned adaptations}. The distinction is important, because on-the-spot design modifications which are responsive to partly-unblinded results could lead to increased overall Type I Error, if this is not accounted for. 
Note that CSE as described in~\Cref{sec:cse} 
covered \emph{planned adaptations}. This section will generalize CSE to handle unplanned adaptations at interims.

Some analytic techniques exist to ensure Type I Error control while maintaining flexibility for unplanned changes. A typical approach is to use combination tests, in conjunction with closed testing for multiple tests~\citep{posch2005testing,bretz2009adaptive,wassmer2015designing}.
A more general approach to handling Type I Error for unplanned adaptations is to use \emph{conditional error principle}, which provides Type I Error control under the constraint that $\EEE\br{\phi_{\theta}}$ will not be increased by re-design, where $\phi_{\theta}$ is the false positive indicator function. ~\citep{koenig2008adaptive} [find other references].\todojames{todo}
While~\citet{sklar:2022}[Chapter 5] 
discusses the use of the conditional error framework with proof-by-simulation,
we provide necessary updates and generalizations.

We begin by first discussing the issue of Type I Error control when some design features are unknown, such as enrollment rates. To place this within the CSE framework, we must emphasize the difference between what we call \emph{design parameters}, such as patients or number of interims, and \emph{statistical parameters}, which are connected to the likelihood of outcomes, as we discussed earlier in Section X.\todojames{where?} 
For example, if each patient has a covariate $x_i$, then conditioning on the $x_i$'s treats the covariates as design parameters. But if we instead modeled these $X$'s as drawn from a model $P_{X}(\theta')$, then $\theta'$ is a statistical parameter within the broader model, and the $x_i$ would be outcomes rather than design parameters. The categorization is therefore determined by the likelihood model we choose to focus on. It is usually helpful for reasons of reducing dimensions of the statistical parameters to treat covariates as design parameters, conditioning on them in a sequentially grouped fashion which we describe next.

\subsection{Single-Period Conditioning for Covariates or Unclear Enrollment}\label{appendix:single-period}

Before we introduce the full sequential model, we shall discuss a simplified ``single-period" model. Even in a design with no interims, some design parameters will not be determined at the start (e.g. the enrollment size, times of enrollment, and patient covariates). We must still assume that the likelihood model for outcomes is conditionally valid and that the design plan is pre-specified in sufficient detail that no flexibility of choice remains once these design parameters are known. 

Then, to achieve Type I Error control in this single-period setting, it suffices to run the trial, collect data, and run CSE calibration \emph{conditionally on the design parameters} after they are known. This suffices for overall Type I Error control because CSE calibration will establish Type I Error control conditional on the design parameters, and conditional Type I Error control implies unconditional Type I Error control.

\subsection{Group Sequential Conditioning for Interim Changes and/or Rolling Enrollment}

MIKE: The blow is too complicated and should be its own paper. It would be nice to do this more efficiently, as well, if some of the simulation sets can be dropped! Left for future work.

Next, we consider unplanned changes that occur at an interim analysis, or cases where patient recruitment runs past the first interim. We can iterate-forward the previous conditioning argument, interim-by-interim, with a technique we will refer to as \textit{group sequential conditioning}. 

Let us assume that the latest change to the protocol plan occurred at time $t_0$. We shall call this plan the ``current protocol," and will assume it has been followed until the current time $t$. If the trial ends by time $t$ without the need to change the protocol, then we recover the situation in~\Cref{appendix:single-period}. It must be assumed that the outcome model used for CSE has retained conditional validity up through time $t$.

Next, what if a protocol change is desired? Unplanned modifications could be motivated by failure to enroll sufficient samples, addition of a new arm, or a realization that the outcome model should be changed.
In this case, the design has a ``current plan" for the remainder of the trial, which will be exchanged for a ``new plan." The ``current plan" is used to budget-out the remaining conditional Type I Error, and the ``new plan" must be shown to lie below it. 

A subtle point: while it is necessary for a portion of the plan that \emph{actually occurs} that the protocol is followed and models were well-specified, it is \emph{acceptable} if the initial projected plan for the future from time $t$ onward was based on unrealistic or unachievable projections, or even a wrong model. However, to the extent that the ``new plan" was accurately anticipated as a possibility, the better the resulting power is likely to be. For an example in this vein,~\citet{koenig2008adaptive} considers planning ahead for a chance of dropping the drug at interim for safety reasons.

At the change-point, we will condition on all so-far revealed design parameters up to time $t$, 
and use a variation of CSE as described below in a multi-step process to determine how much Type I Error remains. 
Then, we calibrate the new design to ensure the budget is maintained.
We describe this procedure in more detail.
Let $\set{t_i}_{i=1}^{I}$ be the sequence of times when the design undergoes unplanned changes. Letting $t_0 \equiv 0$, we initially pre-register the protocol for the trial
with a target Type I Error surface of $\alpha_1(\theta) \equiv \alpha$ for $\theta \in \Theta$. Then, our procedure follows a roughly 5-step loop starting from $t_i = t_0$:

\begin{enumerate}[label=(\arabic*)]
\item\label{itm:keep-protocol}
    At time $t_i$, we fix the ``current protocol" which is assumed binding and well-specified until it is changed. 
    Continue the design with outcomes blinded to this algorithm, until the next time $t_{i+1}$ when either the trial is stopped (for success or futility) or the protocol plan is changed.
\item\label{itm:condition}
    At time $t_{i+1}$ when a protocol change occurs, we condition on the next set of design parameters 
    for patients to be revealed, but \emph{not outcomes}, from the time range $t_{i}$ to $t_{i+1}$ (inclusive).
\item
    Given a current Type I Error budgeting function $\alpha_{t_i}(\theta)$ (initialized as $\alpha_{t_0}(\theta) := 2.5\%$), 
    we use CSE to calibrate the protocol, conditionally on the conditional Type I Error surface as of stage ~\labelcref{itm:condition}. Optionally, we may add a `refund' of $\alpha$ unspent by the previous design to this conditional Type I Error surface.
    We arrive at a calibration for the ``current protocol" $\hat{\lambda}_{full}$. 
\item
    Reveal unblinded outcome data for the period from $t_i$ to $t_{i+1}$. If $t_{i+1}$ is an interim during which a rejection could occur, use the calibrated threshold $\hat{\lambda}_{full}$ to perform rejections.
\item
    If $t_{i+1}$ were not the end of the trial, then use a new group of simulations to estimate the remaining conditional Type I Error under the ``current plan" protocol plan to form a new budget $\alpha_t(\theta)$. Then, at the time of the next re-design or the trial's conclusion, $\alpha_t(\theta)$ will be used. We may now return to~\labelcref{itm:keep-protocol}, where the current time $t$ will serves as the next $t_0$.
\end{enumerate}

Informally, why does this approach work? This series of steps maintains a supermartingale condition for the Type I Error under $P_{\theta}$, which will crawl forward by alternately conditioning on ancillary design parameters, and then running the martingale. Taking $M(t)$ as the conditional Type I Error (resolving at $M(\tau) = 1$ for a false rejection or otherwise $M(\tau) = 0$), our initial calibration establishes $M(0)\leq \alpha$. 
We assume that the design parameters for the first interim are assumed known by the filtration $\mathcal{F}_0$.
Then, the supermartingale property implies that $\EEE\br{M(\tau) | \mathcal{F}_0} \leq \alpha$. The final result follows since the true type I Error is equal to the unconditional $E[M(\tau)]$.

To establish Type I Error control more formally, we shall break up this roadmap into further smaller steps, with slightly different notation and definitions.

\begin{algorithm}[H]
\caption{Sequential Recalibration}
\begin{algorithmic}[1]
\State Set $t_0 = 0$. Pre-register the initial protocol for the trial.
\State Initialize a target Type I Error surface $\alpha_1(\cdot): \Theta_0 \subset R^d \rightarrow [0,1]$. Usually, this is $\alpha_1(\theta) = 2.5\%$.
\For{$i=1,\ldots,$}
    \State Reveal design parameters from time $t_{i-1}$ to $t_i$.
    \State For a statistical parameter grid $\theta_j$ with associated tiles $H_j$, perform simulations on the ``current protocol." The simulation dataset should be pre-filled with observed outcomes up to time $t_{i-1}$ and design parameters up to time $t_i$. Thus, CSE simulations start with a partly-filled data matrix, and can fill in both unknown outcome data and unknown complete rows (for not-yet-enrolled patients). Note that for patients enrolled between $(t_{i-1}, t_i]$ these simulation may use real-data baseline covariates but in-silico outcomes, replacing the blinded NA's in the data matrix. Unknown design parameters and corresponding future outcome data are also projected and filled in for times greater than $t_i$, adding new complete rows to the data matrix.
    \State The above simulations are used with CSE calibration to determine a calibration $\hat{\lambda}_j$ for every tile $j$, targeting a Type I Error bound of $\alpha_{i}(\theta_j)$ valid over each tile $H_j$. We require that $\alpha$ takes on its worst case on one of the corners of $H_j$; a sufficient condition is that $\alpha$ is quasi-convex over the interior of each $H_j$.
    \State Select $\hat{\lambda}^*_{i} = \min \limits_j \hat{\lambda}_{j,i}$ to be the chosen design calibration.
    \State Reveal outcome data from the period $(t_{i-1}, t_i]$, while following the protocol's logic for stopping and rejections using the calibrated choice $\hat{\lambda}^*_{i}$ up through time $t_i$. If this results in the end of the trial, exit the loop.
    \State If we are continuing beyond $t_i$ we must be doing a design change. Then, at each simulation point $\theta_j$, we perform $L$ new simulations of the (old) ``current protocol" with the design $\hat{\lambda}^*_{i}$, conditioned on all data up to time $t_i$. Therefore, compared to the simulations in Step 5, this step's simulations will have more pre-filled outcome data but the same number of pre-filled rows.
    \State Determine $V_j$, the fraction of simulations which resulted in a false rejection under $\theta_j$ in the previous step, which gives an unbiased estimate of the conditional Type I Error at $\theta_j$.
    \State Define a new target Type I Error surface $\alpha_{i+1}(\cdot): \Theta_0 \subset R^d \rightarrow [0,1]$ which is flat over each $H_j$ and has the property: over $H_j$, $\alpha_{i+1}(\theta)$ is equal to the maximum of the inverted Tilt-bound over $H_j$, with target point $\theta_j$ with value $V_j/L$. %   (c) $\alpha_{i+1}(\theta_j)$ is therefore umbrella-shaped over $H_j$ by the Tilt-bound with a maximum at $\theta_j$ and a minimum achieved at one of the corners of $H_j$ by quasi-convexity
    %(d) In fact, notice b is the only one of these letters that does anything; so we could just state it carefully with a well-described inverted tilt-bound over $H$, and then we can simply notice that (a) and (c) follow!
    \State Pre-register the next protocol to be followed starting from time $t_i$.
\EndFor
\end{algorithmic}
\end{algorithm}

\newpage

It is also possible to modify this procedure by noticing that away from the worst-case tile(s), the Type I Error budget is often not entirely spent by the minimization-and-selection that occurs at step 8; this spare alpha is not under risk and can be kept for future use, which may provide minor flexibility or reduction in simulation costs. An expanded version incorporating this adjustment is possible, for example by using extra simulation step to make an unbiased estimate of the slack, although it is beyond our current scope. % in Appendix X, without proof. Below, we provide proof without the budget adjustment.
\bigskip 

Proof of Type I Error control for Algorithm 3:

The sequential recalibration process is best understood as an application of the \textit{conditional error principle} \cite{koenig2008adaptive}. We shall construct a super-martingale $M_t(\theta)$ which essentially maintains a conditional Type I Error budget. At every point $\theta \in \Theta$, we shall show that a supermartingale property is maintained with respect to a filtration $F_{(i,s)}$ with $(i,s)$ ordered in lexicographic order, with $i \in N^+$ representing the index of the current loop, and $s = 1, 2, 3, 4$ representing key stages, such that $F_{(i,1)}$ is understood to reveal to results of the current loop $i$ up to step 5, $F_{(i,2)}$ reveals the results of the current loop $i$ up to step 8, $F_{(i,3)}$ reveals the results of the current loop $i$ up to step 9, and $F_{(i,4)}$ reveals the results of the current loop $i$ up to step 12. Initialization begins with $M_{0}(\theta) = \alpha_0(\theta)$ with the empty sigma-algebra $F_0$, and the first step will be to $F_{(1,1)}$. Because of this initialization to $\alpha(\theta)$, and because at the conclusion $M$ will resolve to an indicator of false rejection $\phi(\theta)$, optional stopping implies that $E[\phi] \leq \alpha(\theta)$, which is the overall Type I Error guarantee we seek. 

Thus, inductively, it suffices to show that the supermartingale property will be preserved at every advancement to the next $F_{(i,s)}$. Below we define how $M$ evolves and establish the supermartingale property as we move to each value of $s \in \{1, \ldots, 4\}.$

\begin{itemize}
    \item $s=1$. When advancing to step $(1,1)$, $M_0(\theta)$ = $\alpha_1(\theta)$. Inductively when advancing to $i > 1$, the previous loop will have set $M_{i-1,4}(\theta) = \alpha_i(\theta)$. We will not change $M$, and simply set $M_{i,1}(\theta) = M_{i-1,4}(\theta) = \alpha_{i}(\theta)$. The supermartingale property is trivially preserved.

    \item $s=2$. When advancing to step $(i,2)$, we have at the previous step $M_{i,1}(\theta)$ = $\alpha_i(\theta)$. Define $M_{i,2}(\theta) = 1$ if a false rejection occurs under $\theta$, $M_{i,2}(\theta) = 0$ if the trial stops without false rejection, and otherwise the trial continues and we may set $M_{i,2}(\theta)$ to the true conditional Type I Error of $\hat{\lambda}^*$ under the calibrated plan $\hat{\lambda}_i^*$ given $\mathcal{F}_{(i,2)}$. 
    Let $\phi_i$ be the indicator for the event of false rejection under a probability space which assumes correctness of the model used for simulations (i.e., assuming correctness of the outcome model and future projections of the protocol). [We require correctness of this model up until time $t_i$, and will deviate from it after this point]. \todojames{we should probably introduce a more careful definition of this sequence of different probability spaces. The actual history is constructed from different sequential slices! Should perhaps define sigma-algebras $G_i$ carrying forward each successive probability model, and note that $F$ rides along with $G_i$ at step $i$, then hops to the next.}
    Assuming $\alpha_i(\theta)$ is constant over each $H_j$, the arguments of ~\Cref{ssec:calibration:point} - ~\Cref{ssec:calibration:general} can be applied to the budgeting function $\alpha_i(\theta)$ to show that the re-calibrated design is conservative at all points in $\Theta$, and hence $E[\phi_i | \mathcal{F}_{(i,2)}] \leq \alpha_i(\theta)$ where $\phi_i$ is an indicator for the event of false rejection if one were to follow the protocol model calibrated at stage $i$. The conditional Type I Error of the selected design is $M_{i,2}(\theta) = E[\phi_i | \mathcal{F}_{(i,2)}]$. By an application of the tower property of conditional expectation, we arrive at the supermartingale property for this step: $E[M_{i,2}(\theta)|\mathcal{F}_{(i,1)}] \leq M_{i,1}(\theta).$

    \item $s=3$. We have from before that $M_{i,2}(\theta) = E_{\theta}[\phi_i | \mathcal{F}_{(i,2)}]$. We shall define $M_{i,3}(\theta) = E_{\theta}[\phi_i | \mathcal{F}_{(i,3)}]$, which maintains the super-martingale property via the tower property of conditional expectation.

    \item $s=4$. We have from before that $M_{i,3}(\theta) = E[\phi_i | \mathcal{F}_{(i,3)}]$. What occurs in steps 11-12 is an empirical estimation of this conditional Type I Error at $\theta_0$ the center of the tile. In fact, this is similar to the result of ~\Cref{ssec:calibration:general}, except the tilt-bound here is being used in the \textit{other direction}, i.e. using the simulation point as the target rather than originator. 
    
    %To prove that this will work, we can consider that $V$ has a binomial distribution; and then we could construct a test $\rho$ such that with $P(V=v)$, we tune it as $\rho = \rho_v$ with level exactly $V/L$. Then the average positive chance is $E[\rho] = E[\phi_i]$. And, our $M$ is essentially taking a different Tilt-bound from each $\rho_v$ depending on the value of $v$.

    Let us now clearly state the goal: using the algorithm's definition of $\alpha_{i+1}$, in order to maintain the super-martingale condition, we must establish:
    $$E[\alpha_{i+1}(\theta) | \mathcal{F}_{(i,3)} ]\leq E_{\theta}[\phi_i | \mathcal{F}_{(i,3)}]$$. 

    For brevity, below we suppress this notationally as $E_{\theta_0}[\phi_i].$

    Lemma: consider $V$ as binomial random variable with $N=L, p= E_{\theta_0}[\phi_i]$, adjoined independently to the sample space. I claim that (possibly adjoining an extra random variable to the space to assist with random splitting) it is possible to partition $\phi_i$ into pieces $\phi_v$ (suppressing $i$ to avoid writing $\phi_{i,v}$) such that $\phi_v \in \{0,1\}$, and $\phi_v \mathbbm{1}\{V \neq v\} =0$, and $\phi_i = \sum \limits_{v=0}^L \phi_v$, and also such that $E_{\theta_0}[\phi_v] = \frac{v}{L}P(V=v)$. 
    
    Allowing for adjoining of another source of randomness, it is always possible to split an indicator with total probability mass $M$ into a collection of disjoint indicators with masses $m_i$ such that $\sum m_i = M$. Thus, the above partition can be achieved because their probabilities sum to $E[\phi_i]$ due to the expectation formula for the binomial.
    
    (End of helper lemma) 

    \bigskip

    Now, we have the partition $\phi_i = \sum \limits_{v=0}^L \phi_v$. Therefore, we also have

    $E_{\theta}[\phi_i] = \sum \limits_{v=0}^L E_{\theta}[\phi_v] = \sum \limits_{v=0}^L P(V=v)E_{\theta}[\phi_v|V=v]$

    This means the sub-martingale property will be maintained if we can ensure that $$\alpha_{i+1}(\theta) | V=v \leq E_{\theta}[\phi_v|V=v]$$

    Note that $V$ was generated independently of the data that will actually resolve $\phi_i$, and $\phi_v = \mathbbm{1}\{V=v\} \phi_i$. So we my say (by conditional probability) that

    $$E_{\theta_0}[\phi_v|V=v] = \frac{\frac{v}{L} P(V=v)}{P(V=v)} = \frac{v}{L}$$.

    Thus, when simulation at $\theta_0$ yields the result $V=v$, it is sufficient to lower-bound 
    $E_{\theta}[\phi_v|V=v]$ based on the knowledge  $E_{\theta_0}[\phi_v |V=v] = v/L$.

    The Inverted Tilt-Bound suffices, and provides exactly what we need to bound the expectation under $\theta$ using the expectation under $\theta_0$. QED for the difficult part!

    We then have the property for all $\theta \in H_j$, 
    $E[\alpha_{i+1}(\theta)| \mathcal{F}_{(i,3)}] \leq E_{\theta}[\phi_i | \mathcal{F}_{(i,3)}]$. Hence, defining $M_{i,4}(\theta) =\alpha_{i+1}(\theta)$ we maintain the super-martingale property.

\end{itemize}

How will this be represented for use in code? A user doing this ``after the fact" would need to input (1) a list of times when the unplanned adaptations occurred (2) complete protocol plans for the original protocol, and under each unplanned change (3) complete outcome data.

\bigskip

Below, we copy a modification of the algorithm which attempts to preserve and re-use ``un-spent" alpha. Also, we indicate how the tiling can optionally be split more finely (this is probably possible to do at other steps as well? But simplest to do it at one consistent step.).

\begin{algorithm}[H]
\caption{Sequential Recalibration with Alpha-Refunding}
\begin{algorithmic}[1]
\State Set $t_0 = 0$. Pre-register the initial protocol for the trial.
\State Initialize a target conditional Type I Error surface $\alpha_{1}(\cdot) : \Theta_0 \subset R^{d} \rightarrow [0,1].$ Usually this is $\alpha_1(\theta) = 2.5\%$. (Later, we will define analogous functions $\alpha_{k}(\cdot)$ from $\Theta_0 \subset R^d \rightarrow R$; for simplicity we shall have $\alpha_{k}$ constant over each tile $H_j$.)
\For{$i=1,\ldots,$}
    \State Continue the design until the next time $t_i$ when either the trial is stopped (for success or futility) or the protocol plan will be changed. Reveal design parameters from time $t_{i-1}$ to $t_i$, but do not yet reveal the corresponding outcome data. 
    \State Select a statistical parameter grid $\theta_{i,j}$ with associated tiles $H_{i,j}$ covering $\Theta_0$. Perform simulations on the ``current protocol" pre-initialized with outcome data up to time $t_{i-1}$ and design parameters up to time $t_i$. This means the CSE simulations start with a partly-filled data matrix, and can fill in both unknown outcome data and unknown complete rows (for not-yet-enrolled patients). Each simulation must fill in outcomes between $(t_{i-1}, t_i]$, replacing NA's in the data matrix. Unknown design parameters and corresponding future outcome data are also projected and filled in for times greater than $t_i$, adding new complete rows to the data matrix.
    \State The above simulations are used with CSE calibration to determine a calibration $\hat{\lambda}_j$ for every tile $H_{i,j}$, targeting a Type I Error bound of $\alpha_{i}(\theta_j)$ valid over each tile $H_{i,j}$. We require that $\alpha$ takes on its worst case on one of the corners of $H_j$; a sufficient condition is that $\alpha$ is quasi-convex over the interior of each $H_j$.
    \State Select $\hat{\lambda}^*_{i} = \min \limits_j \hat{\lambda}_{j,i}$ to be the chosen design calibration.
    \State (Optional step) Introduce a second set of simulations, independent from sets in Steps X and Y, to estimate conservatively the residual ``unspent alpha" in the previous design plan. \todojames{add more details here! It would also, generally, be nice if we could subsume the previous Algorithm 3 entirely.} Denoting as $K_{i,j}$ the number of simulations performed at $\theta_j$ for this new set of simulation, compute 
    $\beta_{i}(\theta_j) := %\alpha_i(\theta_j) - \frac{1}{K_{i,j} +1} \left(1 + \sum\limits_{k=1}^{K_{i,j}} F_{k,j, \hat{\lambda}_{ij}}(X) \right)$$ 
    \frac{1}{K_{i,j}} \sum \limits_{k=1}^{K_{i,j}} F_{k,j, \hat{\lambda}^*_{i}}(X) - F_{k,j, \hat{\lambda}_{ij}}(X).$ and then set $\gamma_{i,j}$ to be the inverted Tilt-bound over $H_j$, with target equal to $\beta_{i}(\theta_j)$ at $\theta_j$. Skipping this step is equivalent to setting $\gamma=0$.
    \State Reveal outcome data from the period $(t_{i-1}, t_i]$, while following the protocol's logic for stopping and rejections using the calibrated choice $\hat{\lambda}^*_{i}$ up through time $t_i$. If this results in the end of the trial, exit the loop.
    \State If we are continuing we must be doing a design change. Then, we perform a third set of simulations: at each simulation point $\theta_j$, we perform $L_j$ new simulations of the (old) ``current protocol" with the design $\hat{\lambda}^*_{i}$, conditioned on all data up to time $t_i$. Therefore these simulations will have more fixed outcome data, but not more fixed complete rows, than in the previous simulation step.
    \State Determine $V_j$, the number of these new simulations which resulted in a false rejection under $\theta_j$ in Step 11. Thus, $V_j/L_j$ is an unbiased estimate of the conditional Type I Error at $\theta_j$.
    \State Define a new target Type I Error surface $\alpha_{i+1}(\theta)$, as a flattened-over-$H_j$ object with the property: over $H_j$, $\alpha_{i+1}(\theta)$ is equal to the maximum of the inverted Tilt-bound over $H_j$, with target point $\theta_j$ and target value $\frac{V_j(\theta)}{L}$. Then, simply add  $\gamma_{i}(\theta_j)$ to $\alpha(\theta)$ over each corresponding $H_j$ as an offset.
    \State Pre-register the next protocol to be followed starting from time $t_i$.
\EndFor
\end{algorithmic}
\end{algorithm}

\newpage 
\newpage

Proof of modified version with new alpha refund:

This process is best understood as an adaptation of the \textit{conditional error principle}. (add cite; we can pull this citation from koenig2008.) We shall construct a super-martingale $M_t(\theta)$ which essentially maintains a conditional Type I Error budget. At every point $\theta \in \Theta$, we shall show that a supermartingale property is maintained with respect to a filtration $F_{(i,s)}$ with $(i,s)$ ordered in lexicographic order, with $i \in N^+$ representing the index of the current loop, and $s = 1, 2, 3, 4$ representing key stages, such that $F_{(i,1)}$ is understood to reveal to results of the current loop $i$ up to step 6, $F_{(i,2)}$ reveals the results of the current loop $i$ up to step 9, $F_{(i,3)}$ reveals the results of the current loop $i$ up to step 10, and $F_{(i,4)}$ reveals the results of the current loop $i$ up to step 12. Initialization begins with $M_{i,s}(\theta) = \alpha_0(\theta)$ with the empty filtration, and will progress at the next step $F_{(1,1)}$. Because of this initialization to $\alpha(\theta)$, and because at the conclusion $M$ will resolve to an indicator of false rejection $\phi(\theta)$, optional stopping implies that $E[\phi] \leq \alpha(\theta)$, which is the overall Type I Error guarantee we seek. 

Thus, inductively, it suffices to show that the supermartingale property will be preserved at every advancement to the next $F_{(i,s)}$.

\begin{itemize}
    \item $s=1$. Base case $i=1$: When advancing to step $(1,1)$, $M_0(\theta)$ = $\alpha_1(\theta)$. Inductive case $i > 1$:  the previous loop will have already set $M_{i-1,4}(\theta) = \alpha_i(\theta)$. We will not change $M$, and simply set $M_{i-1,4}(\theta) = M_{i,1}(\theta)$. So the supermartingale property is trivially preserved.

    \item $s=2$. When advancing to step $(i,2)$, we have at the previous step $M_{i,1}(\theta)$ = $\alpha_i(\theta)$. Define $M_{i,2}(\theta) = 1$ if a false rejection occurs under $\theta$, $M_{i,2}(\theta) = 0$ if the trial stops without false rejection, and otherwise the trial continues and we may set $M_{i,2}(\theta)$ to the true conditional Type I Error of $\hat{\lambda}^*$ under the calibrated plan $\hat{\lambda}_i^*$ given $\mathcal{F}_{(i,2)}$. Assuming $\alpha_j(\theta)$ is constant over each $H_j$, the arguments of [Calibration Section Proof X] can be applied to the budgeting function $\alpha_j(\theta)$. The tile-wise calibrated $\hat{\lambda}_{i,j}$ is conservative at all points in $H_j$, and hence $E[\phi_{i,\hat{\lambda}_{i,j}}| \mathcal{F}_{(i,1)}] \leq \alpha_i(\theta)$ where $\phi_{i,\lambda}$ is an indicator for the event of false rejection if one were to follow the protocol calibrated to $\lambda$ at stage $i$ (assuming correctness of all of its embedded future planning assumptions). Then, notice that $\gamma_{i,j} \leq E[\phi_{\hat{\lambda}_{i,j}} -\phi_{\lambda^*_i} | \mathcal{F}_{(i,2)}]$
    We shall define the next supermartingale stage as $M_{i,2}(\theta) = E[\phi_{\lambda^*_i} + \gamma_{i,j}| \mathcal{F}_{(i,2)}]$. The supermartingale property $E[M_{i,2}(\theta)|\mathcal{F}_{(i,1)}] \leq M_{i,1}(\theta)$ then follows from an application of the tower property of conditional expectation.

    \item $s=3$. We have from before that $M_{i,2}(\theta) = E_{\theta}[\phi_{\lambda^*_i} + \gamma_{i,j}| \mathcal{F}_{(i,2)}]$. We shall define $M_{i,3}(\theta) = E_{\theta}[\phi_{\lambda^*_i} + \gamma_{i,j}| \mathcal{F}_{(i,3)}]$, which maintains the super-martingale property via the tower property of conditional expectation.

    \item $s=4$. We have from before that $M_{i,3}(\theta) = E[\phi_{\lambda^*_i} + \gamma_{i,j}| \mathcal{F}_{(i,3)}]$. What occurs in step 8 is an empirical estimation of this conditional Type I Error at $\theta_0$ the center of the tile. In fact, this is similar to the result as [Proof of validity for a single tile in the calibration process using the inverted tilt-bound], except the tilt-bound here is being used in the \textit{other direction}, i.e. using the simulation point as the target rather than originator. 
    
    %To prove that this will work, we can consider that $V$ has a binomial distribution; and then we could construct a test $\rho$ such that with $P(V=v)$, we tune it as $\rho = \rho_v$ with level exactly $V/L$. Then the average positive chance is $E[\rho] = E[\phi_i]$. And, our $M$ is essentially taking a different Tilt-bound from each $\rho_v$ depending on the value of $v$.

    Let us try to clearly state the goal: We shall aim to show (using the algorithm's definition of $\alpha_{i+1}$):
    $$E[\alpha_{i+1}(\theta) | \mathcal{F}_{(i,3)} ]\leq E_{\theta}[\phi_{\lambda^*_i} + \gamma_{i,j}| \mathcal{F}_{(i,3)}]$$. 

    Notice that $\gamma_{i,j}$ is simply functioning as a constant offset. Below, we will show $E[\alpha_{i+1}(\theta) - \gamma_{i,j}| \mathcal{F}_{(i,3)}] \leq E_{\theta}[\phi_{\lambda^*_i}| \mathcal{F}_{(i,3)}]$

    Lemma: consider $V$ as binomial random variable with $N=L, p= E_{\theta_0}[\phi_{\lambda^*_i}]$, adjoined independently to the sample space. We claim that (possibly adjoining another random variable to the space for random splitting) it is possible to partition $\phi_{\lambda^*_i}$ into pieces $\phi_v$ (suppressing $i$ to avoid writing $\phi_{i,v}$) such that $\phi_v \in \{0,1\}$, and $\phi_v 
 = \mathbbm{1}\{V=v\} \phi_v$, and $\phi_i = \sum \limits_{v=0}^L \phi_v$, and also such that $E_{\theta_0}[\phi_v] = \frac{v}{L}P(V=v)$.
 
 It is generally always possible to split an indicator with total probability mass $M$ into a collection of other indicators with masses $m_i$ such that $\sum m_i = M$. Thus, our above partitioning can be done, because the sum of these disjoint sets' probabilities matches up with $E[\phi_i]$ due to the expectation formula for the binomial.

    \bigskip

    Now, we have the partition $\phi_{\lambda^*_i} = \sum \limits_{v=0}^L \phi_v$. Therefore, we also have

    $E_{\theta}[\phi_{\lambda^*_i}] = \sum \limits_{v=0}^L E_{\theta}[\phi_v] = \sum \limits_{v=0}^L P(V=v)E_{\theta}[\phi_v|V=v]$

    This means the sub-martingale property will be maintained if we can ensure that $$\alpha_{\theta} | V=v \leq E_{\theta}[\phi_v|V=v]$$

    Note that $V$ was generated independently of the data that will actually resolve $\phi$, and $\phi_v = \mathbbm{1}\{V=v\} \phi_v$. So we my say (by Bayes' Rule) that

    $$E_{\theta_0}[\phi_v|V=v] = \frac{\frac{v}{L} P(V=v)}{P(V=v)} = \frac{v}{L}$$.

    Thus, when simulation at $\theta_0$ yields the result $V=v$, it is sufficient to upper-bound 
    $E_{\theta}[\phi_v|V=v]$ based on the knowledge  $E_{\theta_0}[\phi_v |V=v] = V/L$.

    The inverted tilt-bound suffices, and provides exactly what is required bound the expectation under $\theta$ using the expectation under $\theta_0$. QED for the difficult part!

    We then have the property for all $\theta \in H_j$, 
    $E[\alpha_{i+1}(\theta)| \mathcal{F}_{(i,3)}] \leq E_{\theta}[\phi_{\lambda^*_i} + \gamma_{i,j}| \mathcal{F}_{(i,3)}]$. Hence, defining $M_{i,4}(\theta) =\alpha_{i+1}(\theta)$ we maintain the super-martingale property.
\end{itemize}
